# Supplementary material for: Multi-Objective Molecule Generation using Interpretable Substructures
Source: arXiv:2002.03244 source file (2020-07-02)
Supplement: Supplementary file 1 [file appendix.tex]

\newpage
\appendix
\onecolumn
\section{Technical Details}

\textbf{Rationale Distribution } The optimal solution of $P(\gS)$ in Eq.(\ref{eq:ratdist}) is derived as follows. Let the training objective 
\begin{equation}
    \gL = \sum_\graph\nolimits \mathbb{I}[\graph] P(\graph) + \lambda \mathbb{H}[P(\gS)]
        = \sum_\graph\nolimits \mathbb{I}[\graph] \sum_\gS\nolimits P(\graph | \gS) P(\gS) - \lambda \sum_\gS\nolimits P(\gS) \log P(\gS)
\end{equation} Since $P(\gS)$ is a categorial distribution, the optimal $P(\gS)$ should satisfy $\frac{\partial \gL}{\partial P(\gS)} = 0$ for all $\gS$. Specifically,
\begin{equation}
\frac{\partial \gL}{\partial P(\gS_k)} = \sum_\graph\nolimits \mathbb{I}[\graph] P(\graph | \gS_k) - \lambda P(\gS_k) - \lambda = 0 \quad \Rightarrow \quad P(\gS_k) \propto \exp\left(\frac{1}{\lambda} \sum_\graph\nolimits \mathbb{I}[\graph] P(\graph | \gS_k)  \right)
\end{equation}
To compute $P(\gS_k)$, we approximate the inner expectation $\sum_\graph \mathbb{I}[\graph] P(\graph | \gS_k)$ with 20 samples of molecules $\graph$.

\section{Experimental Details}

\textbf{Hyperparameters } For MCTS rationale extraction, we set exploration constant $c_{puct}=10$ and maximum rationale size $N=20$. For graph completion, the hidden dimension of encoder and decoder MPN is 400 and latent dimension $|\vz|=20$. For rationale distribution, we set $\lambda = 0.02$. As a result, the probability mass is mostly concentrated on rationales $\gS_k$ with the highest expected reward $\sum_\graph \mathbb{I}[\graph] P(\graph | \gS_k)$. This does not hurt output diversity as long as there are many such rationales. 

For REINVENT, we pre-train their prior network on the ChEMBL dataset, which contains 1.02 million molecules. We use their default hyperparameters except $\sigma=60$, which is necessary for achieving high success rate on multi-property tasks. We use their official implementation for our experiments (\url{github.com/MarcusOlivecrona/REINVENT}).

For GCPN, we use their default hyperparameters in their official implementation (\url{github.com/bowenliu16/rl_graph_generation}), except that their reward function is replaced with our DRD2, GSK3$\beta$ and JNK3 predictors.

\textbf{Toxicity Prediction } The toxicity dataset contains 105K compounds for training and 20K for testing. In total, there are 26.5K toxic molecules and 164 types of structural alerts. We train a graph convolutional network to predict toxicity, which achieves 0.99 AUROC score. Our GCN implementation is based on chemprop package~\citep{yang2019analyzing}. For attribution AUC metric (partial match accuracy), please refer to \citet{mccloskey2019using} for its definition.
